# Supplementary material for: Object-Level Explanations for Image Geolocation Models: a GeoGuessr use-case
Source: arXiv:2605.00912 source file (2026-04-29)
Supplement: Supplementary file 1 [file X_suppl.tex]

\clearpage
